# Supplementary material for: Design of van der Waals Interfaces for Broad-Spectrum Optoelectronics
Source: arXiv:1912.10345 ancillary file (2020-02-04)
Supplement: Supplementary file 1 [file ubrig_final_SI.pdf]

# Supplementary Information: Design of *van der Waals* Interfaces for Broad-Spectrum Optoelectronics

Nicolas Ubrig,[1,2,*] Evgeniy Ponomarev,[1,2] Johanna Zultak,[3,4,5] Daniil Domaretskiy,[1,2] Viktor Zólyomi,[3] Daniel Terry,[3,4,5] James Howarth,[3,4,5] Ignacio Gutiérrez-Lezama,[1,2] Alexander Zhukov,[3,4,5] Zakhar R. Kudrynskyi,[6] Zakhar D. Kovalyuk,[7] Amalia Patanè,[6] Takashi Taniguchi,[8] Kenji Watanabe,[8] Roman V. Gorbachev,[3,4,5] Vladimir I. Fal'ko,[3,4,5,†] and Alberto F. Morpurgo[1,2,‡]

[1]*Department of Quantum Matter Physics, University of Geneva, 24 Quai Ernest Ansermet, CH-1211 Geneva, Switzerland*

[2]*Group of Applied Physics, University of Geneva, 24 Quai Ernest Ansermet, CH-1211 Geneva, Switzerland*

[3]*National Graphene Institute, University of Manchester, Booth St E, M13 9PL, Manchester, UK*

[4]*School of Physics & Astronomy, University of Manchester, Oxford Road, M13 9PL, Manchester, UK*

[5]*Henry Royce Institute for Advanced Materials, M13 9PL, Manchester, UK*

[6]*School of Physics & Astronomy, The University of Nottingham, Nottingham, NG7 2RD, UK*

[7]*Institute for Problems of Materials Science, NAS of Ukraine, Chernivtsi Branch, 5 I. Vilde Str., Chernivtsi 58001, Ukraine*

[8]*National Institute for Materials Science, 1-1 Namiki, Tsukuba, 305-0044, Japan*

---

[*] nicolas.ubrig@unige.ch

[†] Vladimir.Falko@manchester.ac.uk

[‡] alberto.morpurgo@unige.ch

## S1. PHOTOLUMINESCENCE EXCITATION SPECTROSCOPY (PLE)

Photoluminescence excitation spectroscopy (PLE) measurements have been performed on several of the samples presented in the main text, to gain insight on the nature of the dynamics of the photogenerated electron and hole pairs prior to their radiative recombination. The results of the measurements are consistent with the band diagrams discussed in Fig. 4 of the main text, and support our interpretation of the observed interfacial photoluminescence as due to interlayer transitions at Γ.

The behavior representative of the interfaces that we have studied is illustrated in Fig. S1 with data measured on an interface formed by 2L-InSe and 2L-$WS_2$. In the experiments we record the spectrum of the photoluminescence signal in the interface region (in this case in

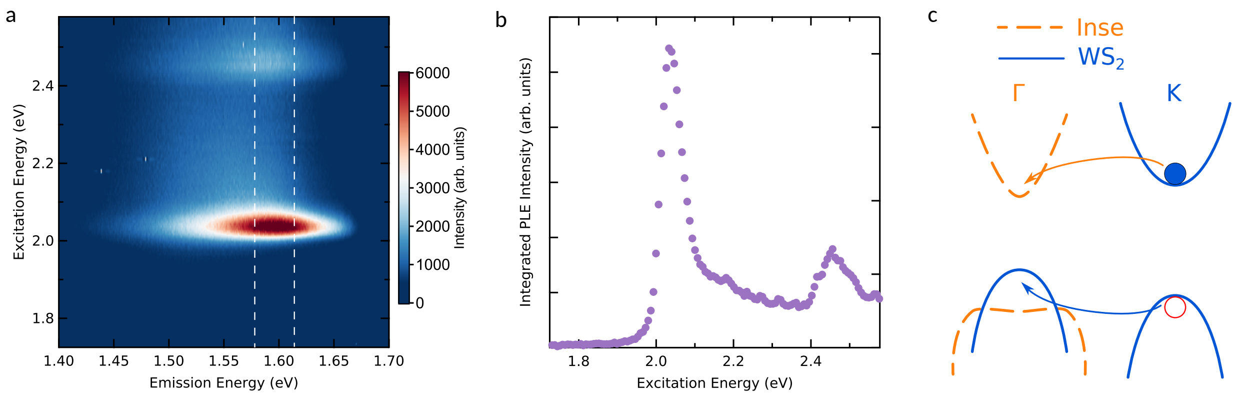


FIG. S1. **a**. Color plot of the PL intensity measured at T = 5 K on a 2L-InSe/2L-$WS_2$ interface, as a function of emitted photon energy (x-axis) and excitation energy of the laser (y-axis). The interface emits at energies close to 1.6 eV. For that energy the PL exhibits two peaks as a function of energy of the excitation laser, at 2.0 eV and 2.5 eV, resulting from the resonant excitation of respectively the A- and the B-exciton at the K-point of 2L-$WS_2$. The phenomenon is illustrated also in panel **b**, where the PL intensity –integrated over the energy interval delimited by the vertical dashed lines in a– is plotted as a function of excitation laser energy. **c**. Schematics of the relevant parts of the band structure of 2L-InSe/2L-$WS_2$ illustrating the charge transfer process leading to the measured PL. The photo-excited electrons and holes at the K-point of $WS_2$ reach the Γ-point (the electron is transferred into InSe, whereas the hole remains in $WS_2$) where eventually they recombine through a radiative interlayer transition.

the spectral region around 1.6 eV, corresponding to the interlayer transition as discussed in the main text (see Fig. 1(c)), while varying the laser excitation energy at constant power. The measured intensity of the PL signal plotted as function of the emitted photon energy and of laser excitation energy is shown in Fig. S1**a** (see also Fig. S1**b**). The intensity of the interfacial PL signal exhibits pronounced maxima when the excitation laser energy is approximately 2 and 2.5 eV, corresponding respectively to the resonant excitation of the A-exciton and B-exciton at the K-point of 2L-$WS_2$. This directly shows that the electron and hole generated from the excitation laser initially reside in 2L-$WS_2$. Only in a subsequent stage, the electron and holes relax to the lowest energy states available. According to the band alignment discussed in the main text –shown again in Fig. S1**c** for convenience– the lowest energy configuration corresponds to having the electron occupying a state at the minimum of the conduction band in InSe, with the hole residing at the maximum of the valence band of 2L-$WS_2$. As both these states are located at $\Gamma$, it is possible for the electron to recombine radiatively with the hole, through an interlayer transition that is direct in k-space. The PLE data presented here therefore show that all steps from photon absorption to photon emission are consistent both with the band diagram of the interface discussed in the main text (see Fig. 4**b** and Fig. S1**c**) and with what is known about the properties of the individual layers (*e.g.* about the details of resonant absorption at the K-point of 2L-$WS_2$).

We have further performed PLE experiments on the lamella sample discussed in the main text (see Fig. 2**d**). In Fig. S2 we show the PL emitted from a 6L-InSe/2L-$WS_2$ interface centered around 1.3 eV, as a function of energy of the excitation laser, for two orthogonal linear polarizations of the laser beam (respectively parallel and perpendicular to the basal plane). A clear difference in the signal is observed only for excitation energies close to 1.6 eV, i.e. in the spectral region corresponding to intralayer absorption in InSe. Indeed, only when the polarization of the exciting laser is perpendicular to the plane, absorption due to an InSe intralayer transition occurs. Electrons and holes are then photogenerated in the InSe layer. Whereas the electrons stay in InSe, the holes can relax their energy and reach the top of the valence band in 2L-$WS_2$, located at $\Gamma$ (see Fig. 4**b**). As a result, the electrons in the conduction band of InSe can radiatively recombine with the relaxed holes, increasing the intensity of the interlayer PL signal. Also these measurements therefore show that all steps from photon absorption to photon emission are consistent with both the band

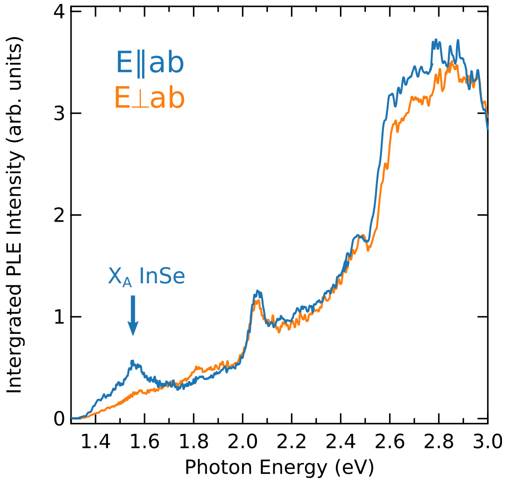


FIG. S2. Intensity of the PL measured at the energy of the emission peak of a 6L-InSe/2L-$WS_2$ interface (1.3 eV) as a function of excitation laser energy. The blue curve corresponds to having the incident excitation laser beam propagating in the interface plane (i.e., ab-plane), with the electric field polarized perpendicular to it. The orange curve corresponds to the case in which the excitation laser propagates in the direction perpendicular to the ab-plane with the electric field polarized in the plane. The only significant difference between the two cases is observed when the energy of the excitation laser beam is around 1.6 eV, corresponding to the energy of the intralayer transition in 6L-InSe. Due to the selection rules of the involved orbitals, this transition is excited only when the electric field is polarized perpendicular to the interface plane. As a result, only in this case electrons and holes are photogenerated by the incoming laser light. Subsequently, the holes are transferred to the Γ-point of 2L-$WS_2$ (see band diagram in Fig. 4**b** of the main text), so that the electrons –which remain in 6L-InSe– can recombine through an interlayer transition, leading to the enhancement of the PL signal observed in the measurements.

diagram of the interface discussed in the main text (see Fig. 4**b**) and with what is known about the properties of the individual layer (i.e., the requirement to induce an intralayer transition in InSe multilayers, namely the need for the polarization of the exciting light to be perpendicular to the InSe layer).

## S2. VALENCE AND CONDUCTION BAND-OFFSETS BETWEEN ***N*L-WS$_2$** AND ***N*L-INSE**

In the main text we have discussed how we extract the value of the interfacial band gap from experiments, which enables the complete band alignment of $N$L-WS$_2$ and $N$L-InSe to be inferred from optical measurements. The analysis of the data also enables the relevant band offsets –i.e., not only the band-gaps– to be estimated. In the tables below we summarize the values of the band offsets that we extracted for all the interfaces discussed in the main text. Positive (Negative) values indicate that the band-edge of the system reported in the column lies above (below) the band-edge of the system reported in the line (compare with Fig. 4 of the main text).

TABLE I. Valence Band Maximum offsets in eV between $N$L-InSe and 2L-$WS_2$.

| | 2L-InSe | 3L-InSe | 4L-InSe | 5L-InSe | 6L-InSe | 7L-InSe |
|---|---|---|---|---|---|---|
| 2L-$WS_2$ ($\Gamma$) | -0.39 | -0.25 | -0.25 | -0.18 | -0.07 | -0.07 |
| 2L-$WS_2$ (K) | -0.19 | -0.05 | -0.04 | 0.03 | 0.13 | 0.13 |

TABLE II. Conduction Band Minimum offsets in eV at the interface between $N$L-InSe and 2L-$WS_2$.

| | 2L-InSe | 3L-InSe | 4L-InSe | 5L-InSe | 6L-InSe | 7L-InSe |
|---|---|---|---|---|---|---|
| 2L-$WS_2$ (K) | -0.13 | -0.333 | -0.40 | -0.44 | -0.46 | -0.48 |

TABLE III. Valence Band Maximum offsets in eV at the interface between $N$L-$WS_2$ and 4L-InSe.

| | 2L-$WS_2$ ($\Gamma$) | 2L-$WS_2$ (K) | 3L-$WS_2$ ($\Gamma$) | 4L-$WS_2$ ($\Gamma$) | 5L-$WS_2$ ($\Gamma$) |
|---|---|---|---|---|---|
| 4L-InSe | 0.24 | -0.04 | 0.31 | 0.30 | 0.3 |

TABLE IV. Conduction Band Minimum offsets in eV at the interface between $N$L-$WS_2$ and 4L-InSe.

| | 2L-$WS_2$ (K/Q) | 3L-$WS_2$ (Q) | 4L-$WS_2$ (Q) | 5L-$WS_2$ (Q) |
|---|---|---|---|---|
| 4L-InSe | 0.42 | 0.26 | 0.19 | 0.13 |

TABLE V. Valence Band Maximum offsets in eV at the interface between 4L-InSe and 2L-TMD.

| | 2L-$MoS_2$ ($\Gamma$) | 2L-$MoS_2$ (K) | 2L-$WS_2$ ($\Gamma$) | 2L-$WS_2$ (K) |
|---|---|---|---|---|
| 4L-InSe | 0.14 | -0.14 | 0.24 | 0.04 |
| | 2L-$MoSe_2$ ($\Gamma$) | 2L-$MoSe_2$ (K) | 2L-$WSe_2$ ($\Gamma$) | 2L-$WSe_2$ (K) |
| 4L-InSe | 0.43 | 0.36 | 0.73 | 0.67 |

TABLE VI. Conduction Band Minimum offsets in eV at the interface between 4L-InSe and 2L-TMD.

| | 2L-$MoS_2$ | 2L-$WS_2$ | 2L-$MoSe_2$ | 2L-$WSe_2$ |
|---|---|---|---|---|
| 4L-InSe | 0.17 | 0.42 | 0.34 | 0.82 |

## S3. ABSOLUTE PL INTENSITY OF THE INTERFACE AND THE CONSTITUENTS

As discussed in the main text, the dependence of the PL signal measured on our TMD-InSe interfaces as function of temperature and laser power is characteristic of interlayer transitions direct in k-space, as expected, since the valence and conduction band edges of

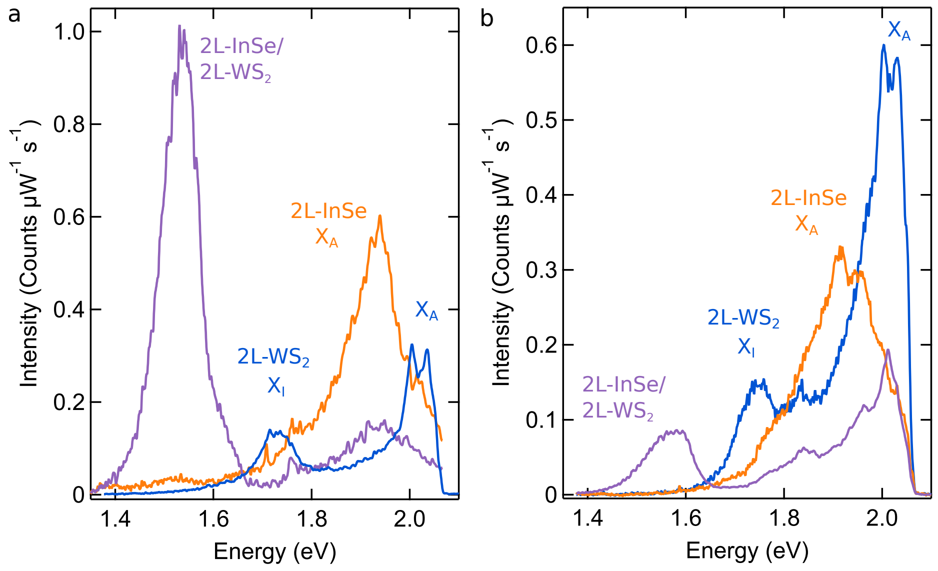


FIG. S3. **a**. Photoluminescence spectra measured at $T = 5$ K on 2L-InSe (orange line), 2L-$WS_2$ (blue line), and on their interface (purple line). The labels on the PL curves measured on the individual InSe and $WS_2$ bilayers refer to the transitions pointed to by the arrows in Fig. 1 of the main text. For this sample the intensity of the interface PL is larger than that of the PL emitted by constituent layers. **b**. Photoluminescence spectra measured on a different 2L-$WS_2$/2L-InSe interface, nominally identical to that shown in **a**. For this device the intensity of the interface PL is smaller than that of the constituent layers. Indeed, we find –as others have found before on interfaces of monolayer TMDs– that the PL intensity of both interface and constituent layers exhibits sizable sample-to-sample fluctuations, as it can be appreciated in the present case by comparing the two different samples shown in panel **a** and **b**.

the constituent layers are centered at Γ. Here we show that these interlayer Γ-Γ transitions –being direct in momentum space– are in principle an efficient light emission process. Indeed, Fig. S2**a** shows that the intensity of such an interlayer transitions (illustrated with data measured on a 2L-$WS_2$/2L-InSe sample at $T = 5$ K), can be brighter than that originating from intralayer transition in the constituent layers. This is an important consideration because, for comparison, the PL intensity in interfaces based on perfectly aligned monolayer TMDs is significantly lower than the PL emission intensity of the bare constituent layers.[S1]

Concerning the absolute emitted intensity, large sample-to-sample fluctuations are ob-

served in all experiments on individual 2D materials, as well as their interfaces (*e.g.*, once again, also on interfaces of aligned TMD monolayers, as well documented in the literature [S1]). The experiments discussed in this work exhibit the same behavior. To illustrate the issue, in Fig. S3**a** and **b** we compare the PL intensity measured on two nominally identical 2L-InSe/2L-$WS_2$ interfaces. It is clear from the data that the observed absolute intensity depends on the specific device measured. It is also clear that this is not a specificity of the interfaces, since comparable sample-to-sample intensity fluctuations are present in the individual layers. For the systems investigated in our work (both constituent layers and interfaces), just as for TMD monolayers and their aligned interfaces reported in the literature,[S1] sample-to-sample variations in PL intensity of nominally identical structures can be as large as two orders of magnitude.

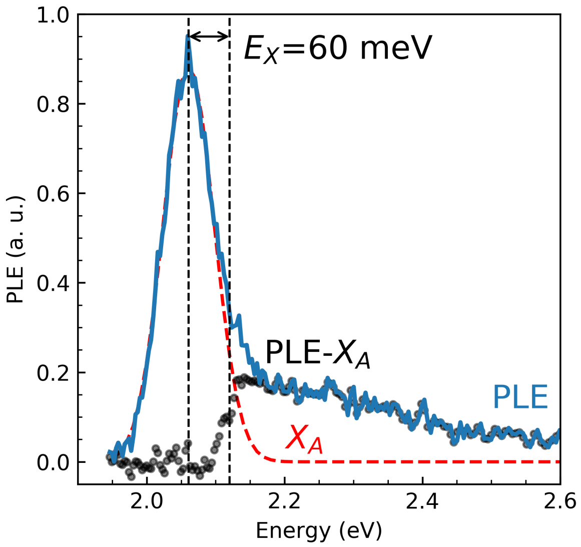


FIG. S4. PLE (solid blue line) from a standing alone InSe bilayer as function of the excitation energy of the laser. The single particle continuum onset (black circles) is obtained by substracting the exciton peak from the PLE curve. The exciton binding energy is simply the difference between the position of the exciton peak (red dashed line) and the onset of the single particle absorption continuum.

## S4. ESTIMATE OF THE INTERLAYER EXCITON BINDING ENERGY

In the main text we have estimated the uncertainty in the energetics of the alignment of the band edges in TMD and InSe multilayers to be 100 meV or better. Part of the uncertainty comes from having neglected the interlayer exciton binding energy in our analysis. To put a bound on this quantity, we note that –owing to their larger spatial extent– interlayer excitons have binding energies that are typically smaller than for intralayer excitons. For InSe multilayers, the exciton binding energy has been recently obtained from PLE measurements, discussed in Ref. S2. For convenience, we reproduce the basic aspects of the data here. The PLE intensity of 2L-InSe as function of the laser excitation energy (see Fig. S4), displays an excitonic peak in the low energy part of the curve, followed by a slow monotonic decay due to single particle absorption. The difference between the peak energy and the onset of the continuum due absorption allows an exciton binding energy of approximately 60 meV to be extracted. Similar experiments –in overall agreement with theoretical calculations– show that the exciton binding energy decreases rapidly with increasing InSe thickness (20 meV for 3L, 18 meV for 4L, 14.5 meV for the bulk).[S2, S3]. The exciton binding energy of $WS_2$ bilayers was also determined experimentally earlier (by means of a different method[S4]), and found to be approximately 80 meV. We can then therefore safely conclude that for 2L-InSe/2L-$WS_2$ interfaces, the interlayer exciton binding energy –being smaller than that of the intralayer excitons in the consituent layers– is certainly significantly smaller than 100 meV. For interfaces based on thicker layers the value of the interlayer exciton binding energy are even much smaller.

---


[S1] A. T. Hanbicki, H.-J. Chuang, M. R. Rosenberger, C. S. Hellberg, S. V. Sivaram, K. M. McCreary, I. I. Mazin, and B. T. Jonker, ACS Nano **12**, 4719 (2018).

[S2] J. Zultak, S. Magorrian, M. Koperski, A. Garner, M. J. Hamer, E. Tovari, K. S. Novoselov, A. Zhukov, Y. Zou, N. R. Wilson, S. J. Haigh, A. Kretinin, V. I. Fal'ko, and R. Gorbachev, arXiv:1910.04215 [cond-mat] (2019), arXiv: 1910.04215.

[S3] J. Camassel, P. Merle, H. Mathieu, and A. Chevy, Physical Review B **17**, 4718 (1978).

[S4] S. Jo, N. Ubrig, H. Berger, A. B. Kuzmenko, and A. F. Morpurgo, Nano Letters **14**, 2019 (2014).
